# Supplementary material for: It Takes Two: Accurate Gait Recognition in the Wild via Cross-granularity Alignment
Source: arXiv:2411.10742 source file (2024-11-16)
Supplement: Supplementary file 1 [file fig_supp_tSNE_cut.pdf]

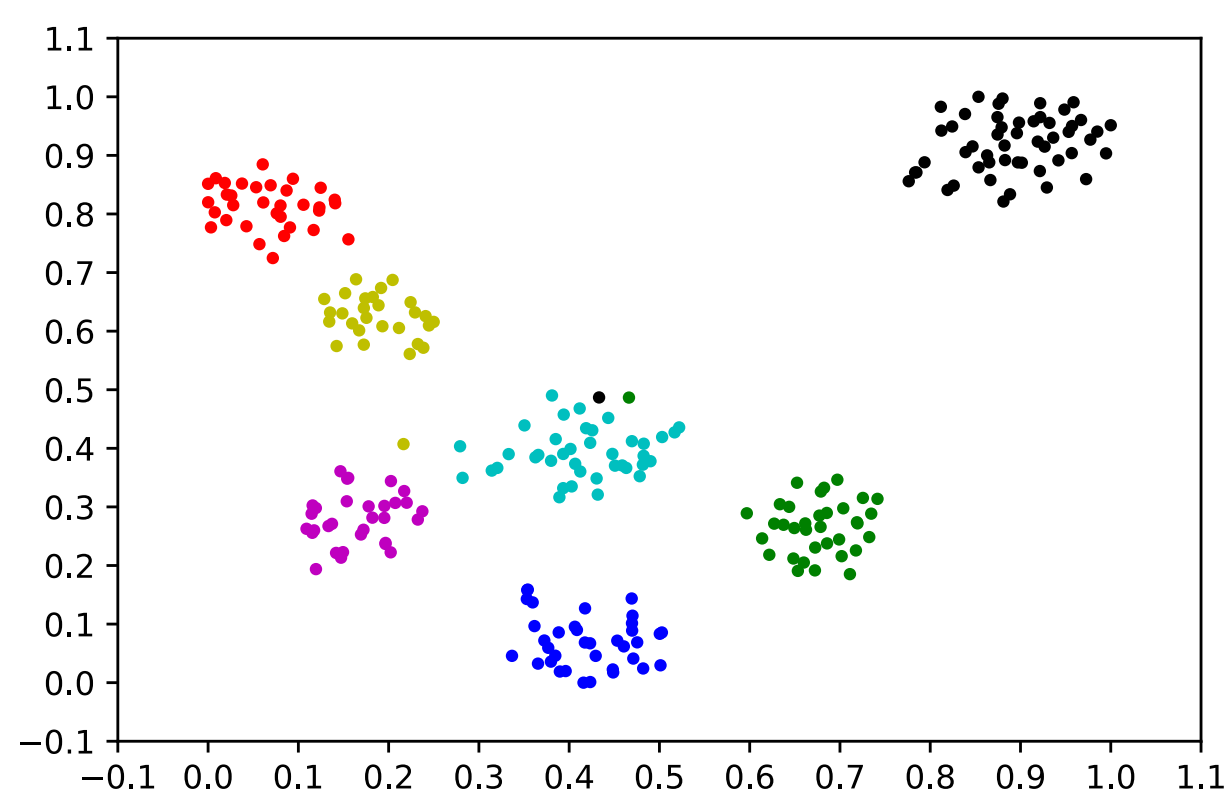

(a) XGait (Only Silhouette)

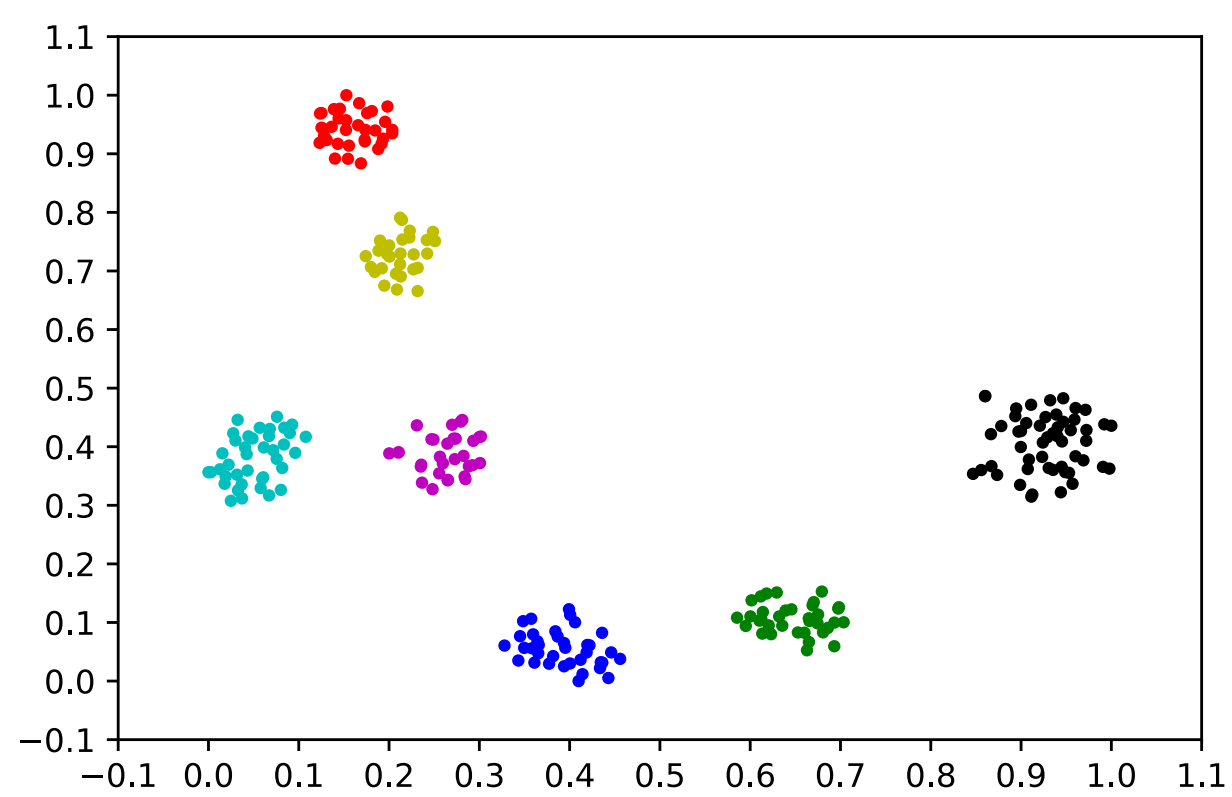

(b) XGait (Only Parsing)

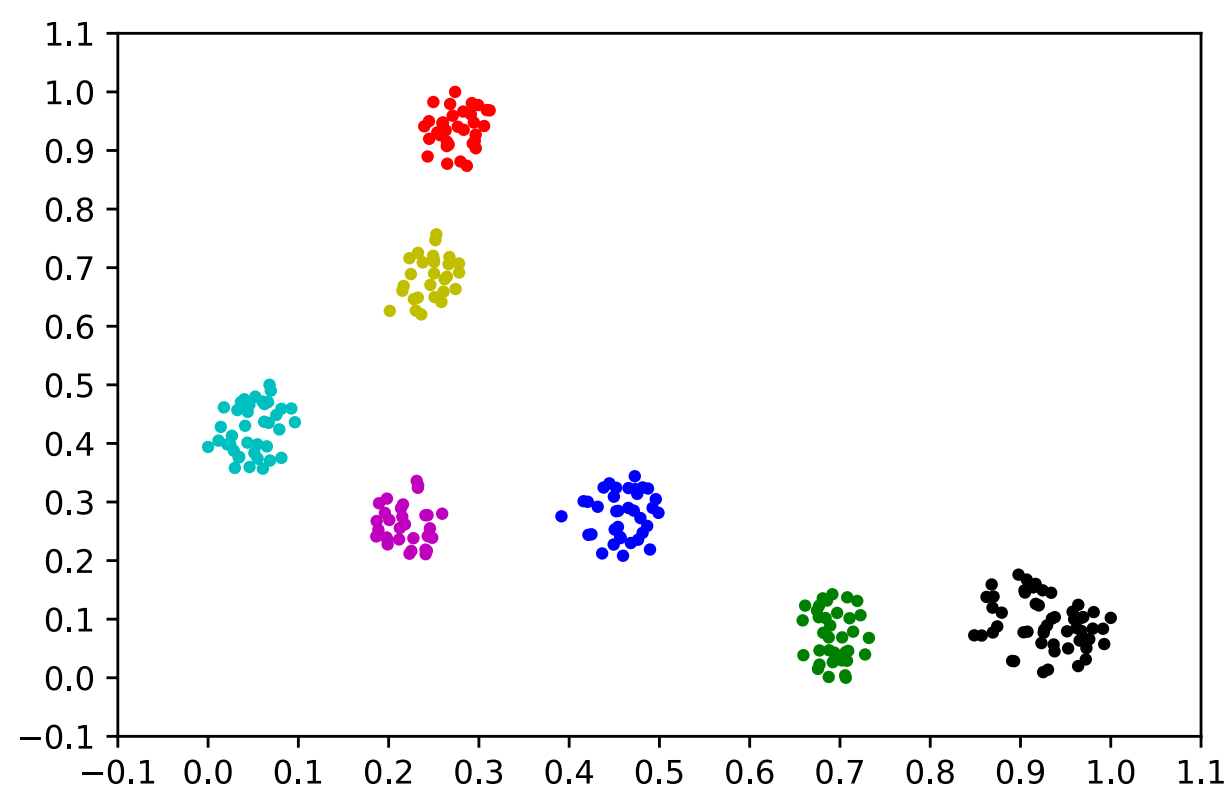

(c) XGait (w/o GCM&PCM)

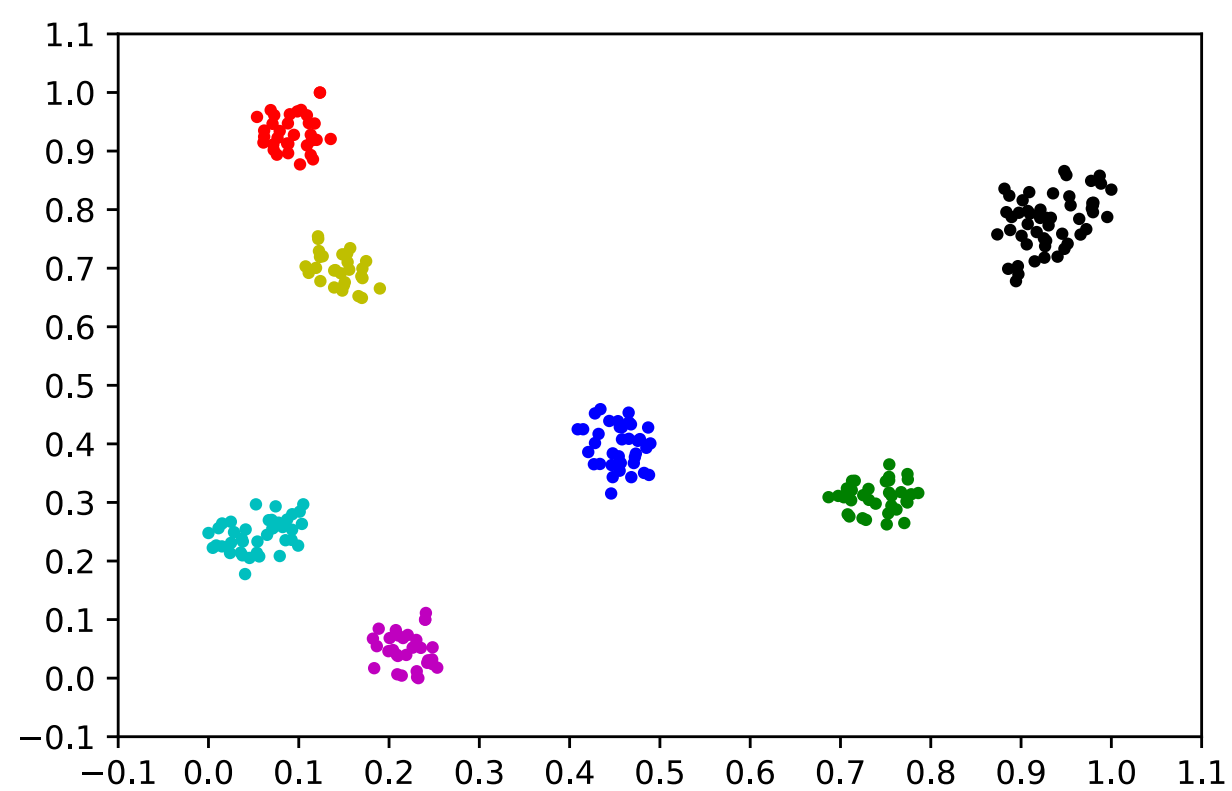

(d) XGait (w/o GCM)

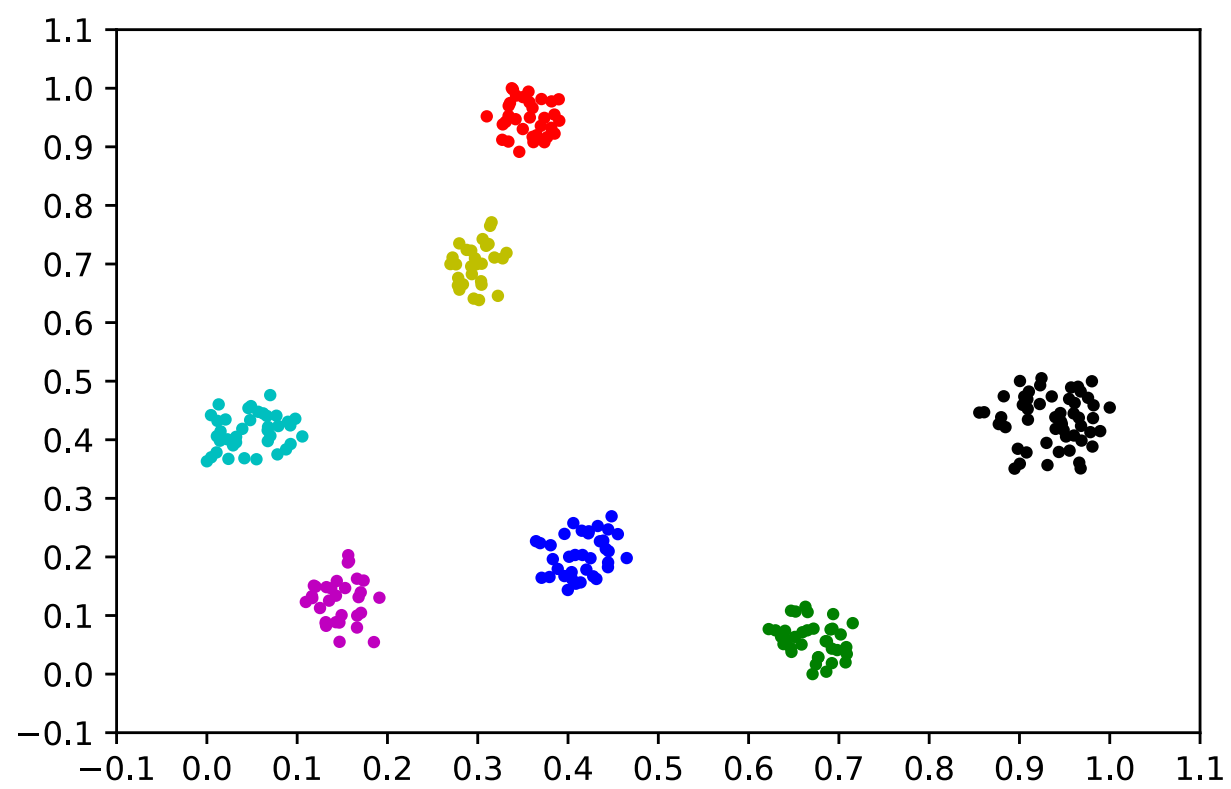

(e) XGait (w/o PCM)

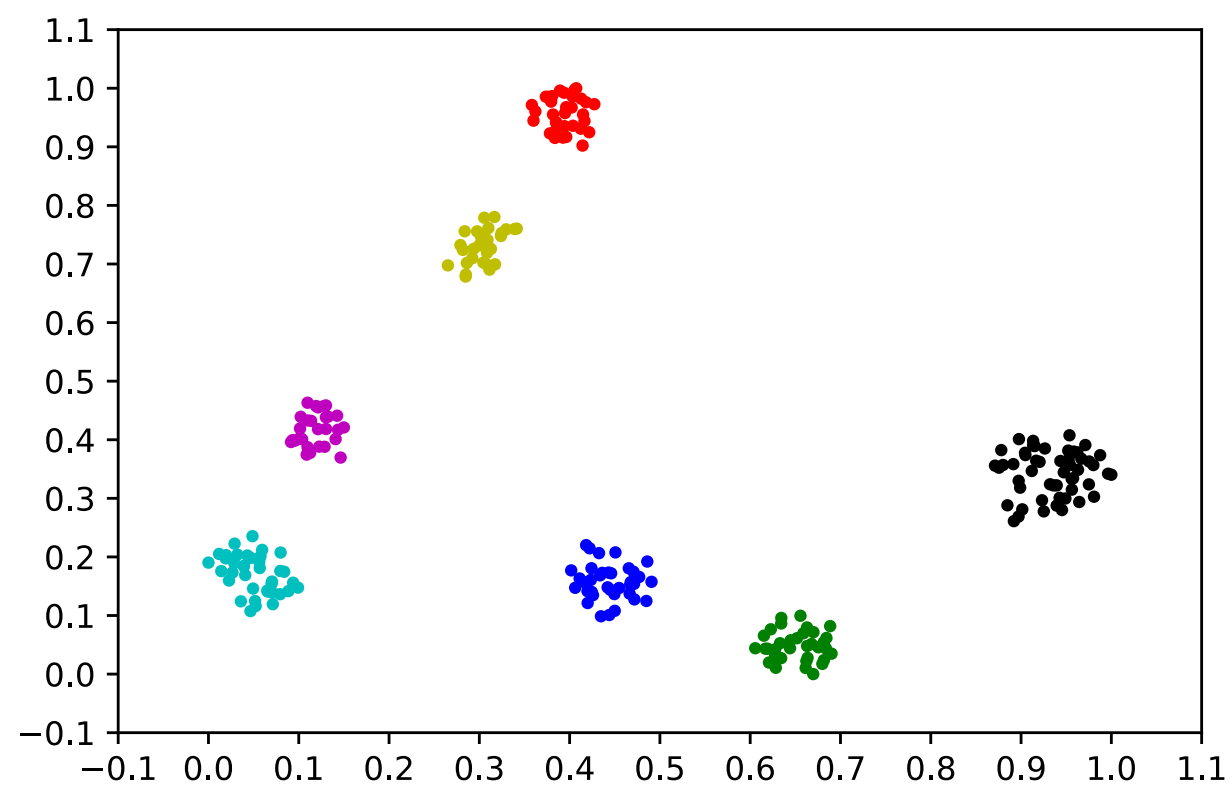

(f) XGait (Ours)

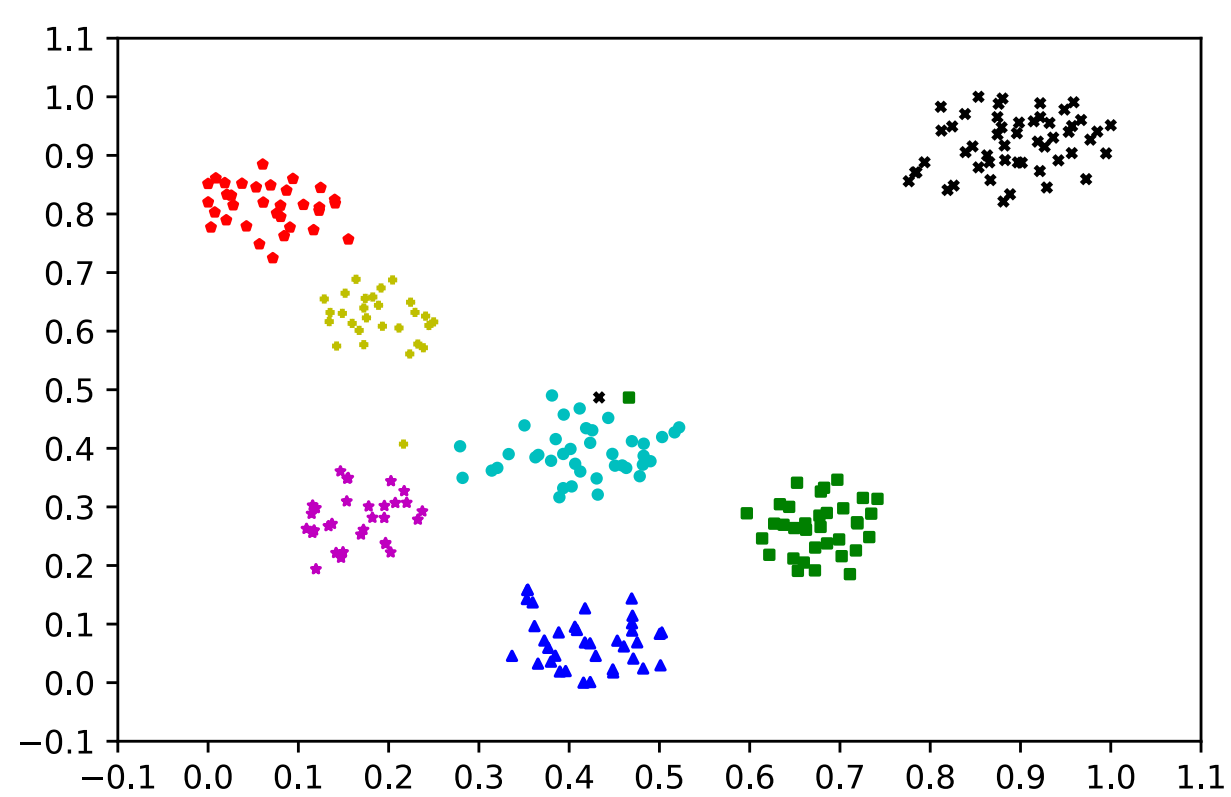

(a) XGait (Only Silhouette)

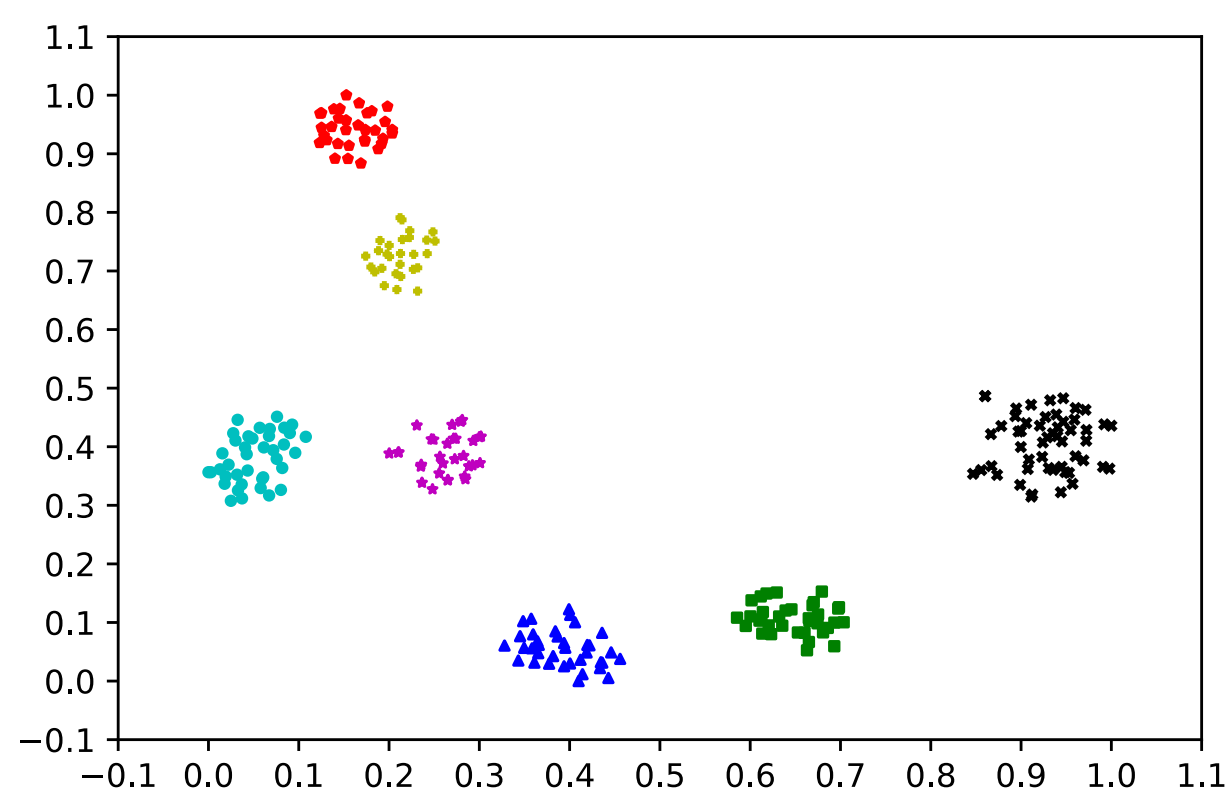

(b) XGait (Only Parsing)

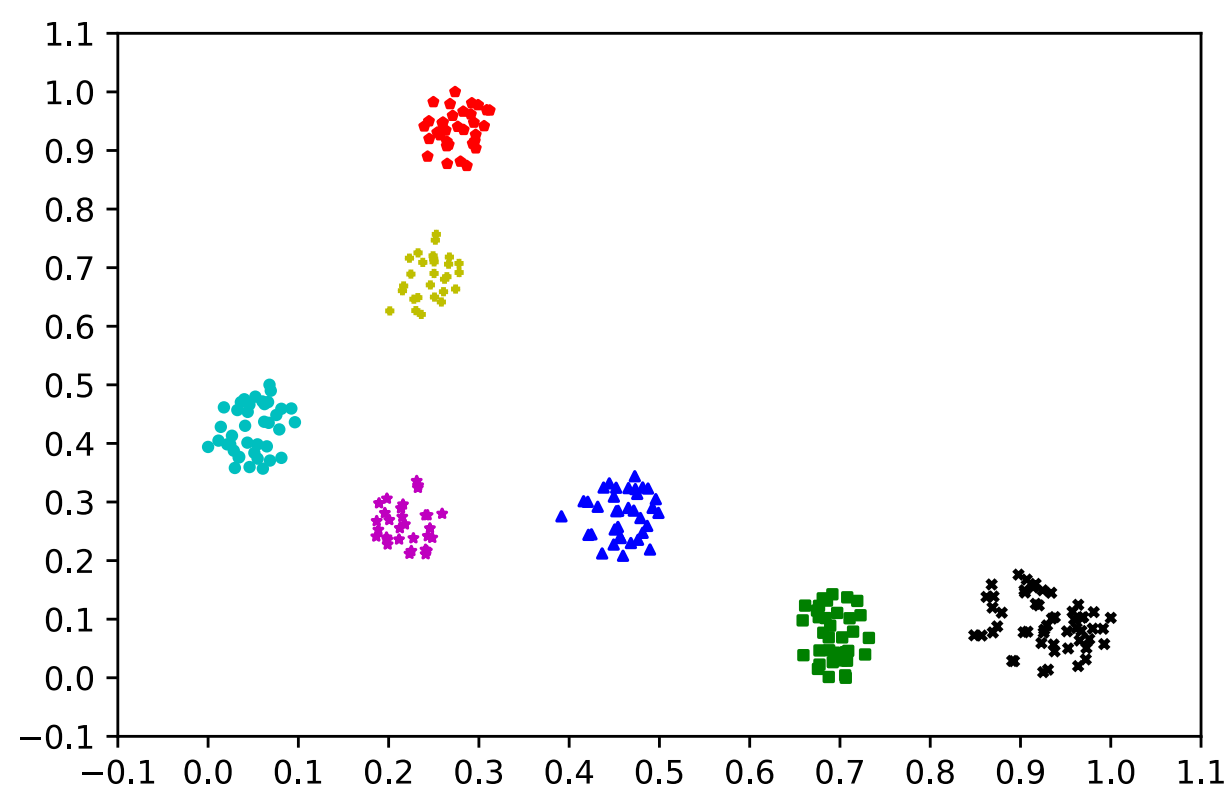

(c) XGait (w/o GCM&PCM)

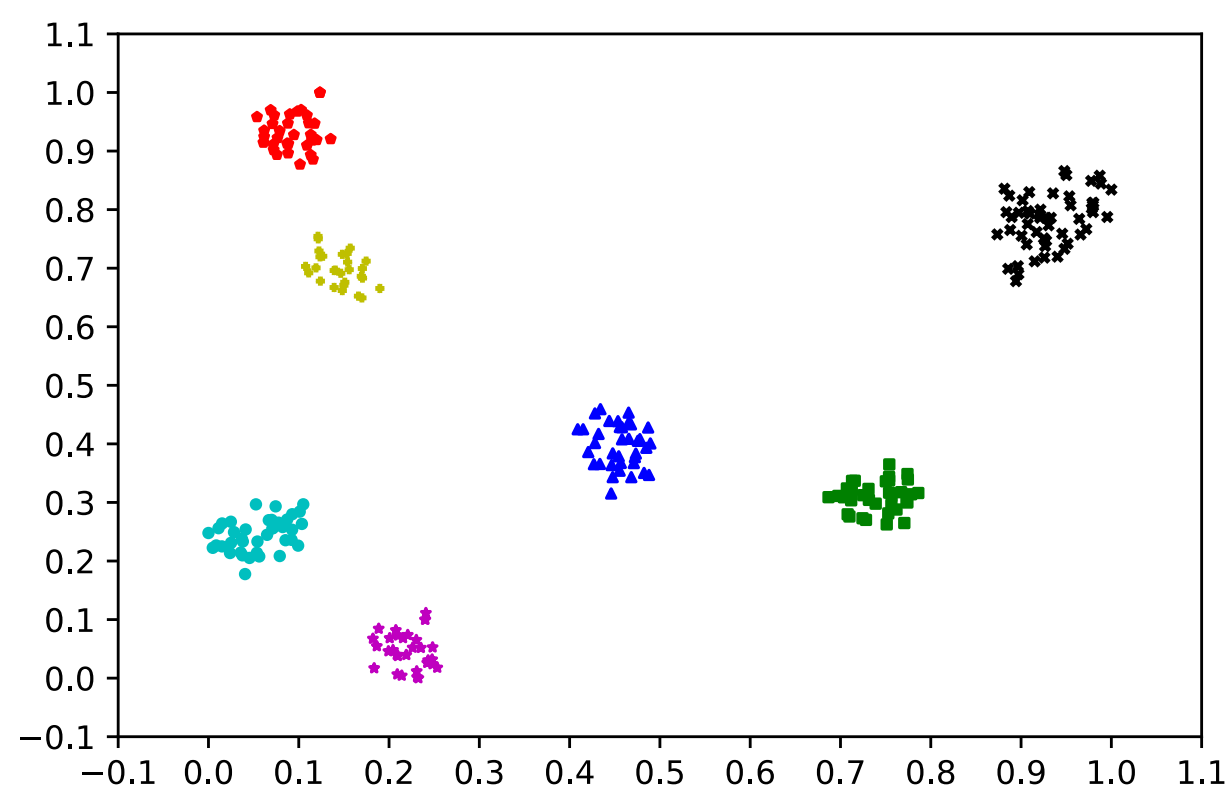

(d) XGait (w/o GCM)

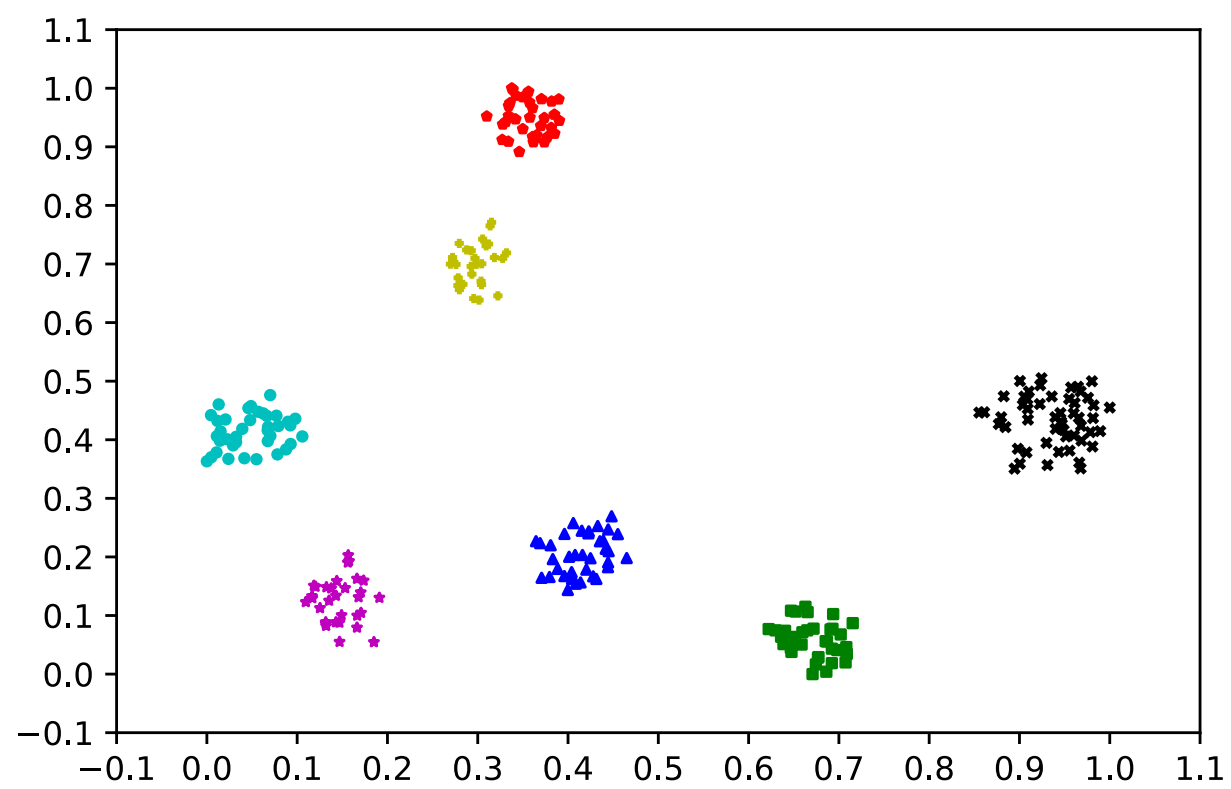

(e) XGait (w/o PCM)

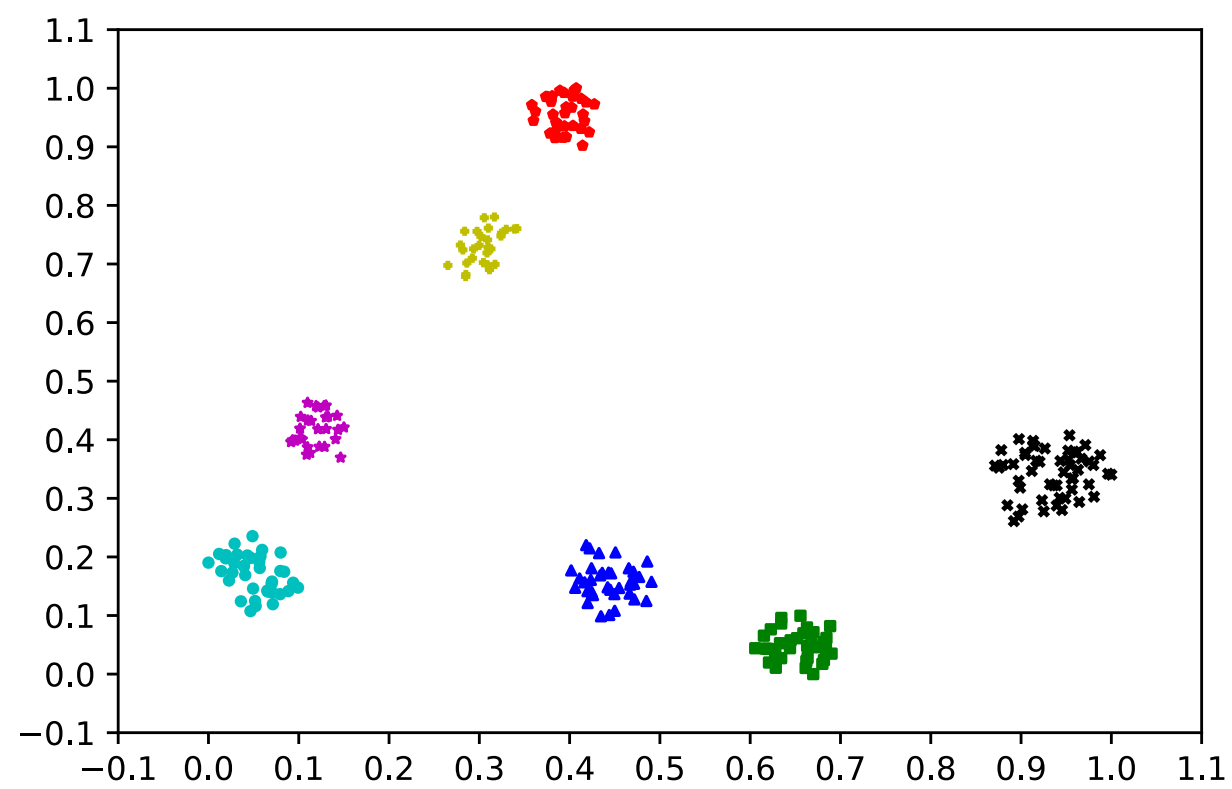

(f) XGait (Ours)

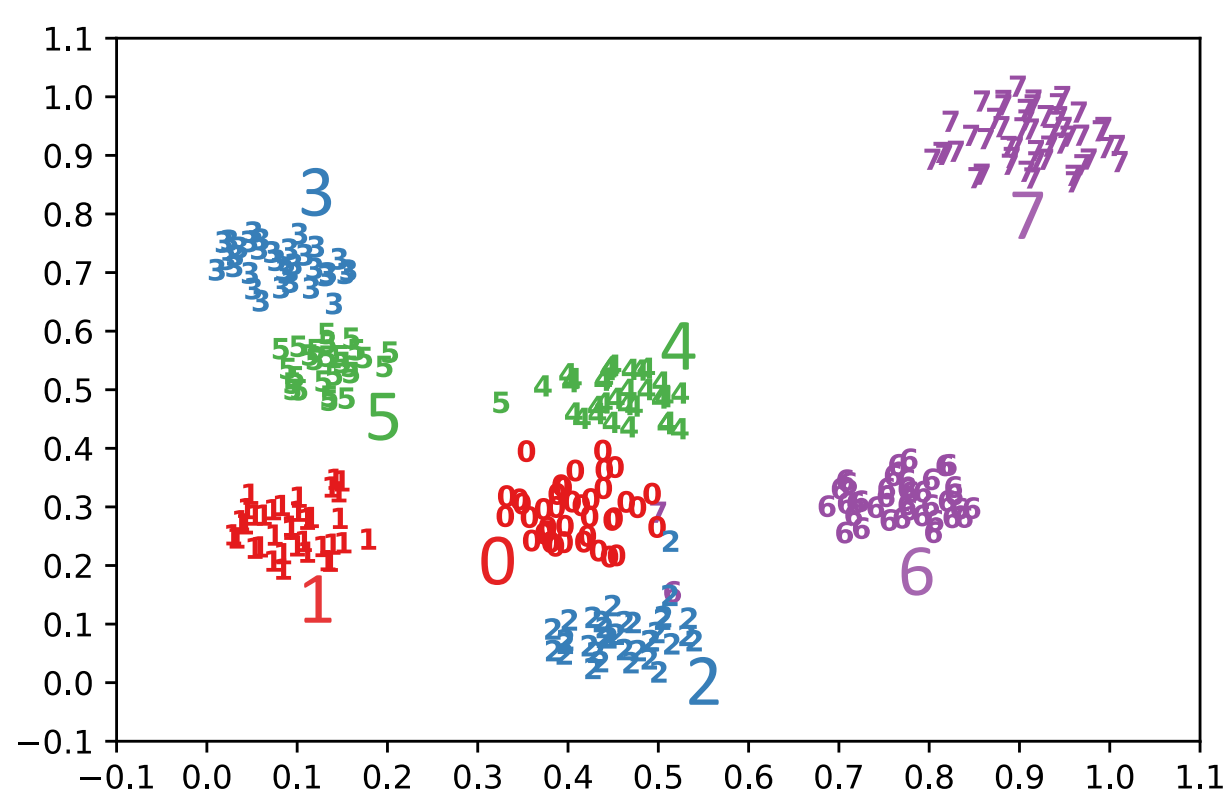

(a) XGait (Only Silhouette)

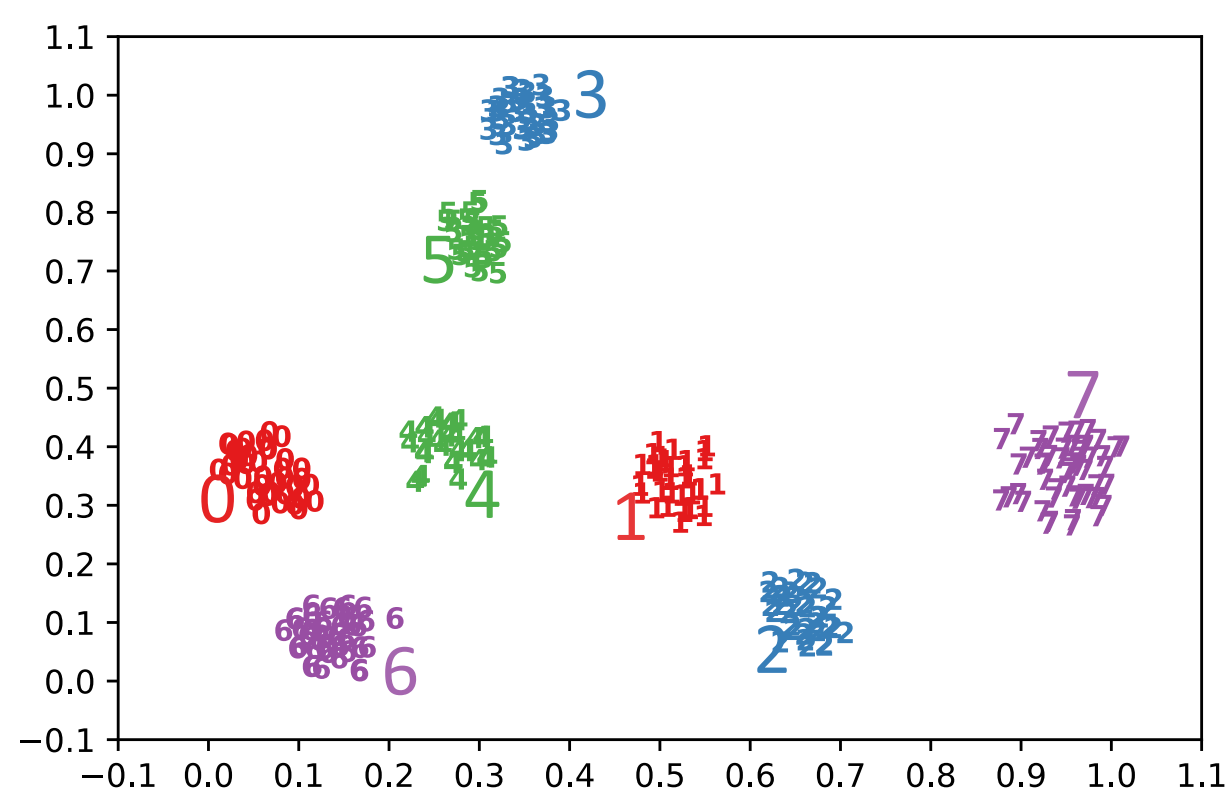

(b) XGait (Only Parsing)

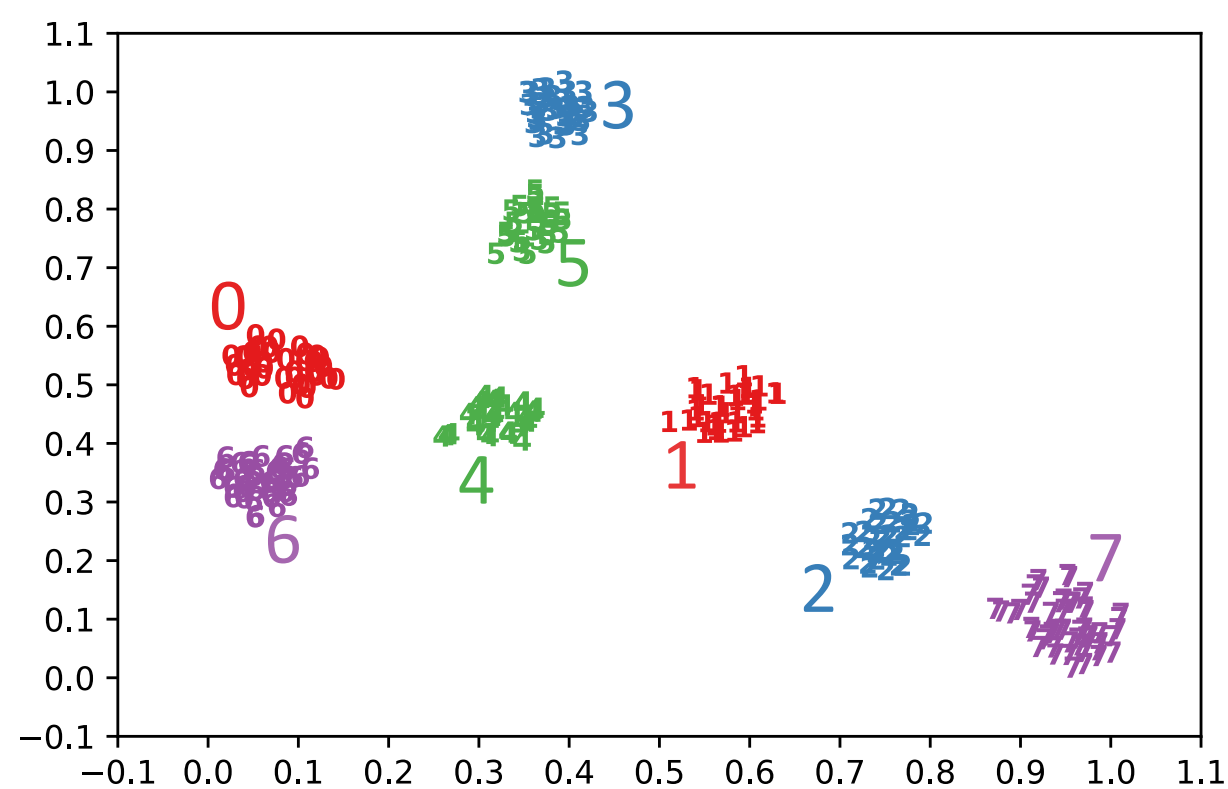

(c) XGait (w/o GCM&PCM)

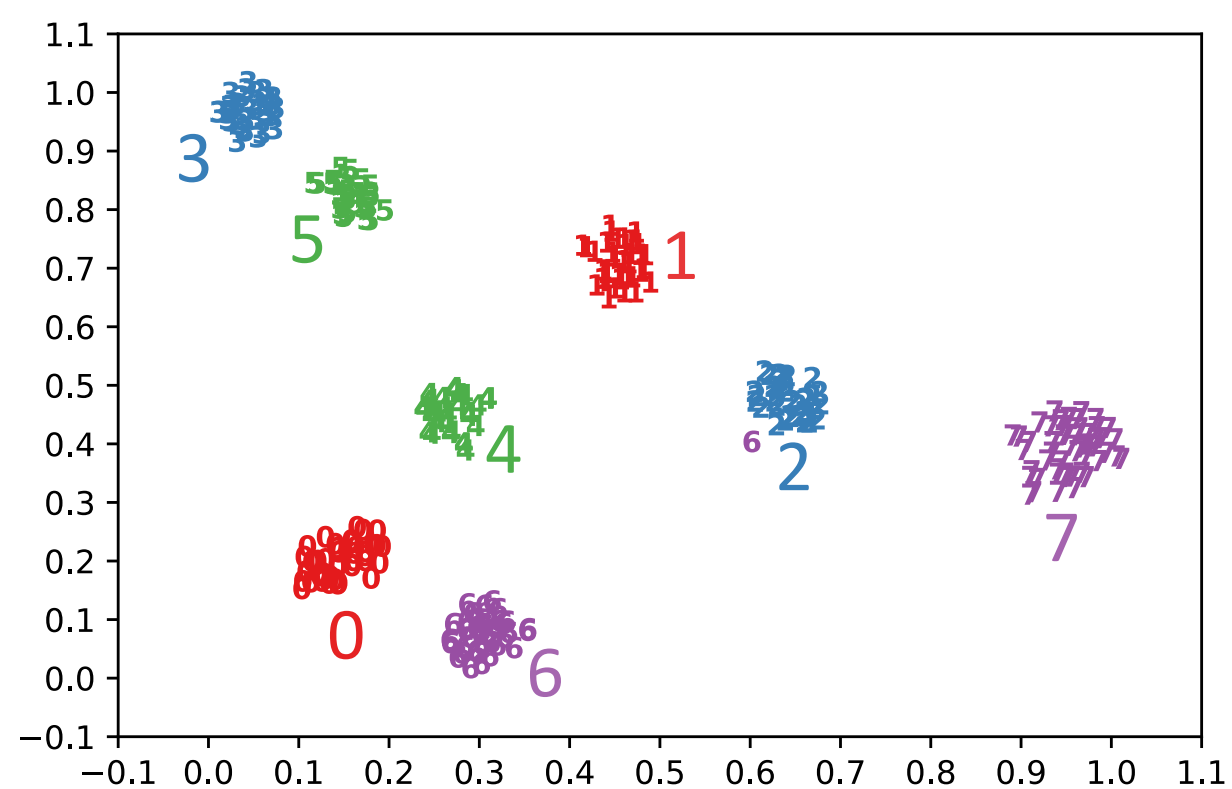

(d) XGait (w/o GCM)

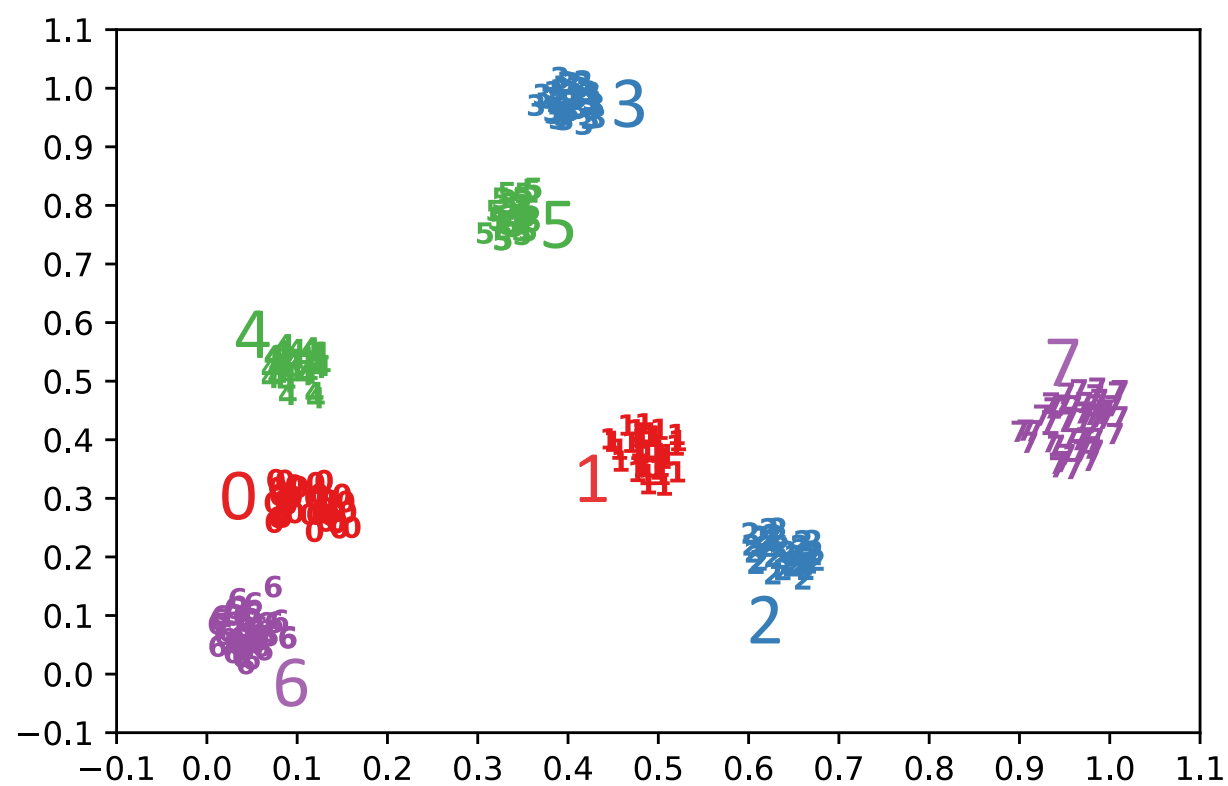

(e) XGait (w/o PCM)

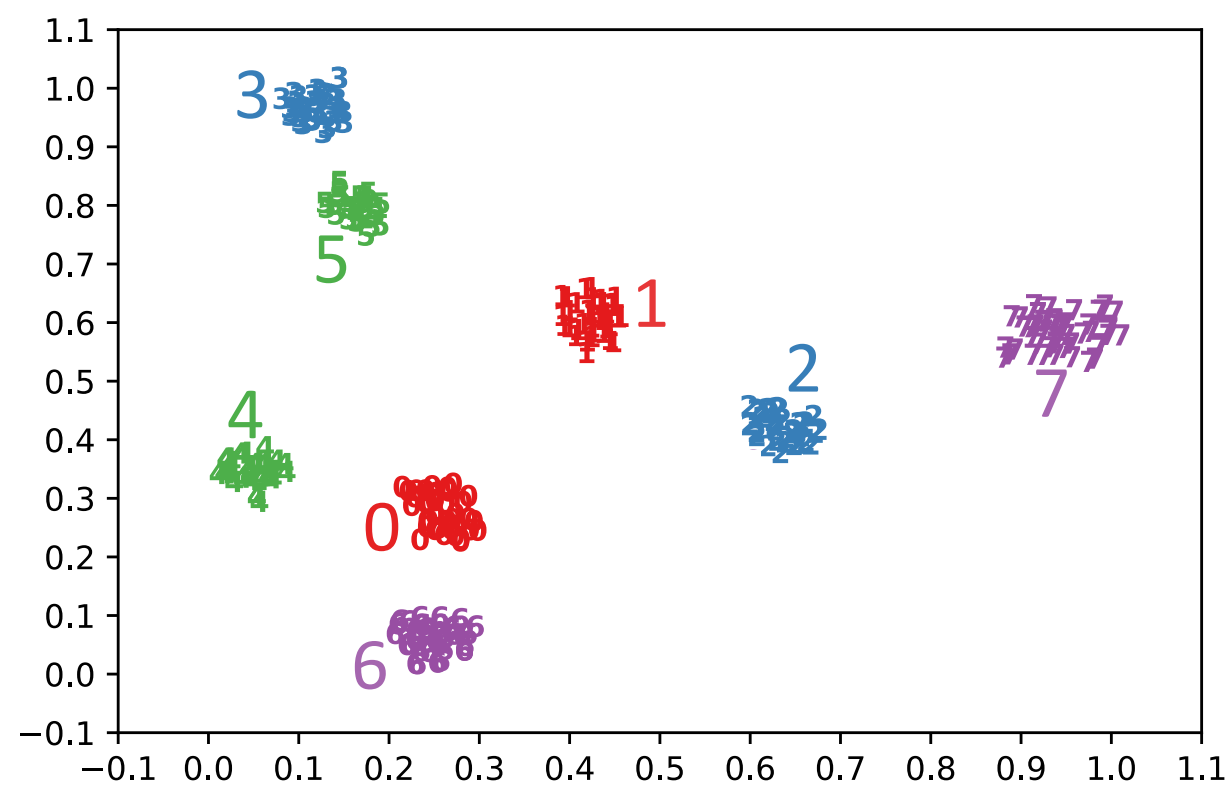

(f) XGait (Ours)
